# Supplementary material for: Binary Fading Interference Channel with No CSIT
Source: arXiv:1405.0203 source file (2017-03-24)
Supplement: Supplementary file 1 [file AppendixLeakage.tex]

In this appendix, we present a variation of Lemma~\ref{Lemma:ConditionalLeakage} for the case of independent channel gains. Consider the scenario where a transmitter is connected to two receivers through binary fading channels as in Figure~\ref{fig:portionHalf}. Suppose $G_i[t]$ is distributed as i.i.d. Bernoulli RV (\emph{i.e.} $G_i[t] \overset{d}\sim \mathcal{B}(p_i)$) where $0 \leq p_2 \leq p_1 \leq 1$, and suppose $G_1[t]$ and $G_2[t]$ are independent. In this channel the received signals are given as
\begin{align}
Y_i[t] = G_i[t] X[t], \qquad i = 1,2,
\end{align}
where $X[t]$ is the transmit signal at time instant $t$. Furthermore, suppose $G_3[t] \overset{d}\sim \mathcal{B}(p_3)$, and 
\begin{align}
& \Pr\left[ G_1[t] = 1, G_3[t] = 1 \right] =  0, \nonumber \\
& \Pr\left[ G_2[t] = 1, G_3[t] = 1 \right] =  0.
\end{align} 
Then, for the channel described above, we have the following lemmas.

\begin{lemma}
\label{lemma:NoCSIT}
{\bf [Conditional Entropy Leakage with Independent Links]} For the channel described above with no CSIT, and for \emph{any} input distribution, we have
\begin{align}
H\left( Y_2^n | G_3^n X^n, G^n \right) \geq \frac{p_2}{p_1} H\left( Y_1^n | G_3^n X^n, G^n \right).
\end{align}
\end{lemma}

\begin{proof} 
Let $G_{h}[t]$ be distributed as $\mathcal{B}(p_2/p_1)$, and be independent of all other parameters in the network. Let
\begin{align}
\bar{Y}_1[t] = G_h[t] Y_1[t], \quad t=1,\ldots,n.
\end{align}

It is easy to verify that $\bar{Y}_1^t$ is statistically the same as $Y_2^t$ under no CSIT assumption, $t=1,\ldots,n$. For time instant $t$ where $1 \leq t \leq n$, we have
\begin{align}
& H\left( Y_2[t] | Y_2^{t-1}, G^t \right) = p_2 H\left( X[t] | Y_2^{t-1}, G_2[t] = 1, G^{t-1} \right) \nonumber \\
& \quad \overset{(a)}= p_2 H\left( X[t] | Y_2^{t-1}, G^t \right) \overset{(b)}= p_2 H\left( X[t] | \bar{Y}_1^t, G^t \right) \nonumber \\
& \quad \overset{(c)}\geq p_2 H\left( X[t] | Y_1^t, G^t \right) \overset{(d)}= \frac{p_2}{p_1} H\left( Y_1[t] | Y_1^{t-1}, G^t \right),
\end{align}
where $(a)$ holds since $X[t]$ is independent of the channel realization at time instant $t$; $(b)$ follows from the fact that $\bar{Y}_1^t$ is statistically the same as $Y_2^t$ under no CSIT assumption; $(c)$ holds since $H\left( \bar{Y}_1^t | Y_1^t, G^t \right) = 0$; and $(d)$ follows from the fact that $\Pr\left[ G_1[t] = 1 \right] = p_1$. Therefore, we have 
\begin{align}
\sum_{t=1}^n{H\left( Y_2[t] | Y_2^{t-1}, G^t \right)} \geq \frac{p_2}{p_1} \sum_{t=1}^n{H\left( Y_1[t] | Y_1^{t-1}, G^t \right)},
\end{align}
and since the transmit signals at time instant $t$ are independent from the channel realizations in future time instants, we have
\begin{align}
\sum_{t=1}^n{H\left( Y_2[t] | Y_2^{t-1}, G^n \right)} \geq \frac{p_2}{p_1} \sum_{t=1}^n{H\left( Y_1[t] | Y_1^{t-1}, G^n \right)},
\end{align}
hence, we get the desired result.
\end{proof}
