# Supplementary material for: Binary Fading Interference Channel with No CSIT
Source: arXiv:1405.0203 source file (2017-03-24)
Supplement: Supplementary file 2 [file AppendixLeakageDelayed.tex]

Let $G_{h}[t]$ be distributed as $\mathcal{B}(p_A/p_B)$, and be independent of all other parameters in the network. Let
\begin{align}
\label{eq:Xh}
X_h[t] = G_h[t] X_B[t], \quad t=1,\ldots,n.
\end{align}

We note that $X_h^t$ is statistically the same as $X_A^t$, $t=1,\ldots,n$; and under the assumptions of the lemma (\emph{i.e.} the transmitter has access to $G_1^{t-1}$ at time instant $t$), the two signals are indistinguishable for the transmitter. 

For time instant $t$ where $1 \leq t \leq n$, we have
\begin{align}
\label{eq:presum}
& H\left( X_A[t] | X_A^{t-1}, G_3^n X^n, G_T^n \right) \nonumber \\
& \quad \overset{(a)}= H\left( X_A[t] | X_A^{t-1}, G_3^n X^n, G_T^n, G_h^{t-1} \right) \nonumber \\
& \quad \overset{(b)}= (1-p_3) H\left( X_A[t] | X_A^{t-1}, G_3^n X^n, G_T^n, G_h^{t-1}, G_3[t] = 0 \right) \nonumber \\
& \quad = p_A H\left( X[t] | X_A^{t-1}, G_3^n X^n, G_T^n, G_h^{t-1}, G_1[t] = 1, G_2[t] = 1, G_3[t] = 0 \right) \nonumber \\
& \quad \overset{(c)}= p_A H\left( X[t] | X_A^{t-1}, G_3^n X^n, G_T^n, G_h^{t-1}, G_1[t] = 1, G_3[t] = 0 \right) \nonumber \\
& \quad \overset{(d)}= p_A H\left( X[t] | X_h^{t-1}, G_3^n X^n, G_T^n, G_h^{t-1}, G_1[t] = 1, G_3[t] = 0 \right) \nonumber \\
& \quad \overset{(e)}\geq p_A H\left( X[t] | X_B^{t-1}, G_3^n X^n, G_T^n, G_h^{t-1}, G_1[t] = 1, G_3[t] = 0 \right) \nonumber\\
% & \quad \overset{(e)}\geq p_A H\left( X[t] | X_B^{t-1}, G_1[t] = 1, G_3[t] = 0, G_3^n X^n, G_T^n, G_h^{t-1} \right) \nonumber\\
& \quad \overset{(f)}= (1-p_3) \frac{p_A}{p_B} H\left( X_B[t] | X_B^{t-1}, G_3^n X^n, G_T^n, G_h^{t-1}, G_3[t] = 0 \right) \nonumber\\
& \quad = \frac{p_A}{p_B} H\left( X_B[t] | X_B^{t-1}, G_3^n X^n, G_T^n, G_h^{t-1} \right) \nonumber\\
& \quad \overset{(g)}= \frac{p_A}{p_B} H\left( X_B[t] | X_B^{t-1}, G_3^n X^n, G_T^n \right),
\end{align}
where $(a)$ holds since $G_h^{t-1}$ is independent of all other parameters in the network; $(b)$ is true due to (\ref{eq:NoTwoEqualToOne}); $(c)$ follows since due to delayed direct-path CSIT assumption, given the realization of $G_1[t]$, the signal is independent of the realization of $G_2[t]$; 
% given 
% \begin{align}
% X_A^{t-1}, G_1[t] = 1, G_3[t] = 0, G_3^n X^n, G_T^n, G_h^{t-1},
% \end{align}
% the signal $X[t]$ is independent of $G_2[t] = 1$;
%from the fact that the signal only depends on realizations of $G_1$; 
$(d)$ holds since 
\begin{align}
& H\left( X[t] | X_A^{t-1}, G_3^n X^n, G_T^n, G_h^{t-1}, G_1[t] = 1, G_3[t] = 0 \right) \nonumber \\
& = H\left( X[t], X_A^{t-1} | G_3^n X^n, G_T^n, G_h^{t-1}, G_1[t] = 1, G_3[t] = 0 \right) - H\left( X_A^{t-1}| G_3^n X^n, G_T^n, G_h^{t-1}, G_1[t] = 1, G_3[t] = 0 \right) \nonumber\\
& = H\left( X[t], X_h^{t-1}| G_3^n X^n, G_T^n, G_h^{t-1}, G_1[t] = 1, G_3[t] = 0 \right) - H\left( X_h^{t-1}| G_3^n X^n, G_T^n, G_h^{t-1}, G_1[t] = 1, G_3[t] = 0 \right) \nonumber\\
& = H\left( X[t] | X_h^{t-1}, G_3^n X^n, G_T^n, G_h^{t-1}, G_1[t] = 1, G_3[t] = 0 \right),
\end{align}
where the second equality holds since $X[t], X_A^{t-1}$ have the same conditional joint distribution as $X[t], X_h^{t-1}$, and $X_A^{t-1}$ has the same conditional joint distribution as $X_h^{t-1}$;
% are the same (in other words, both $X_h^t$ and $X_A^t$ have the same realization of $G_1^{t}$, these signals are indistinguishable for the transmitter); 
$(e)$ is true since from (\ref{eq:Xh}), we know that $X_h^{t-1}$ is a function of $X_B^{t-1}$ and $G_h^{t-1}$;
%\begin{align}
%H\left( X_h^{t-1} | X_B^{t-1}, G_2[t] = 1, G_3^n X^n, G_T^{n}, G_h^{t-1} \right) = 0; 
%\end{align}
% $(e)$ holds since the event $G_2[t] = 1$ is a subset of the event $G_1[t] = 1$; 
$(f)$ follows from the fact that given $G_3[t] = 0$ state $B$ occurs with probability $p_B/(1-p_3)$; and $(g)$ holds since $G_h^{t-1}$ is independent of all other parameters in the network. 

Finally, using (\ref{eq:presum}), we have
\begin{align}
\sum_{t=1}^n{H\left( X_A[t] | X_A^{t-1}, G_3^n X^n, G_T^n \right)} \geq \frac{p_A}{p_B} \sum_{t=1}^n{H\left( X_B[t] | X_B^{t-1}, G_3^n X^n, G_T^n \right)},
\end{align}
which implies
\begin{align}
H\left( X_A^n | G_3^n X^n, G_T^n \right) \geq \frac{p_A}{p_B} H\left( X_B^n | G_3^n X^n, G_T^n \right),
\end{align}
hence, we get the desired result.
