# Supplementary material for: Binary Fading Interference Channel with No CSIT
Source: arXiv:1405.0203 source file (2017-03-24)
Supplement: Supplementary file 3 [file AppendixCorrelation.tex]

Suppose messages $\hbox{W}_1$ and $\hbox{W}_2$ are encoded as $X_1^n$ and $X_2^n$ respectively, and each receiver in the original BFIC can decode its corresponding message with arbitrary small decoding error probability as $n \rightarrow \infty$. 

Now, we show that if we use the same transmission scheme in the BFIC that satisfies (\ref{eq:constraintaa}) and (\ref{eq:constraintbb}), \emph{i.e.}
\begin{align}
\tilde{X}_i[t] = X_i[t], \quad t = 1,2,\ldots,n, \quad i = 1, 2,
\end{align}
then the receivers in the BFIC that satisfies (\ref{eq:constraintaa}) and (\ref{eq:constraintbb}) can still decode $\hbox{W}_1$ and $\hbox{W}_2$.

Note that $X_i[t]$ only depends on $\hbox{W}_i$ and $G_{ii}^{t-1}$, $i=1,2$. Therefore, the error event $\widehat{\hbox{W}}_i \neq \hbox{W}_i$, depends on the choice of $\hbox{W}_i$, $G_{ii}^{n}$, and the marginal distribution of the channel gains $G_{ii}^n$ and $G_{\bar{i}i}^n$. 

Define 
\begin{align}
\mathcal{E}_{\hbox{W}_1} & = \left\{ \left( \hbox{W}_2, G_{12}^n, G_{22}^n \right) \text{~s.t.~} \widehat{\hbox{W}}_1 \neq \hbox{W}_1 \right\}, \nonumber \\
\tilde{\mathcal{E}}_{\hbox{W}_1} & = \left\{ \left( \hbox{W}_2, \tilde{G}_{12}^n, G_{22}^n \right) \text{~s.t.~} \widehat{\hbox{W}}_1 \neq \hbox{W}_1 \right\},
\end{align}
then, the probability of error is given by
\begin{align}
p_{\text{error}} & = \sum_{w_1}{\Pr \left( \hbox{W}_1 = w_1 \right) \Pr \left( \mathcal{E}_{w_1} \right)} \nonumber \\
& = \frac{1}{2^{nR_1}} \sum_{w_1}{\sum_{\left( w_2, g_{12}^n, g_{22}^n \right) \in \mathcal{E}_{w_1}}{\Pr \left( w_2, g_{12}^n, g_{22}^n \right)}} \nonumber \\
& \overset{(a)}= \frac{1}{2^{nR_1}} \sum_{w_1}{\sum_{\left( w_2, \tilde{g}_{12}^n, g_{22}^n \right) \in \tilde{\mathcal{E}}_{w_1}}{\Pr \left( w_2, \tilde{g}_{12}^n, g_{22}^n \right)}} \nonumber \\
& = \tilde{p}_{\text{error}},
\end{align}
where $p_{\text{error}}$ and $\tilde{p}_{\text{error}}$ are the decoding error probability at ${\sf Rx}_1$ in the original and the BFIC that satisfies (\ref{eq:constraintaa}) and (\ref{eq:constraintbb}) respectively; and $(a)$ holds since according to (\ref{eq:constraint}), the joint distribution of $G_{12}^n$ and $G_{22}^n$ is the same as $\tilde{G}_{12}^n$ and $\tilde{G}_{22}^n$ and the fact that the error probability at receiver one only depends on the marginal distribution of these links. Similar argument holds for ${\sf Rx}_2$.
